# Supplementary material for: Integrated Decision Gradients: Compute Your Attributions Where the Model Makes Its Decision
Source: arXiv:2305.20052 source file (2023-12-18)

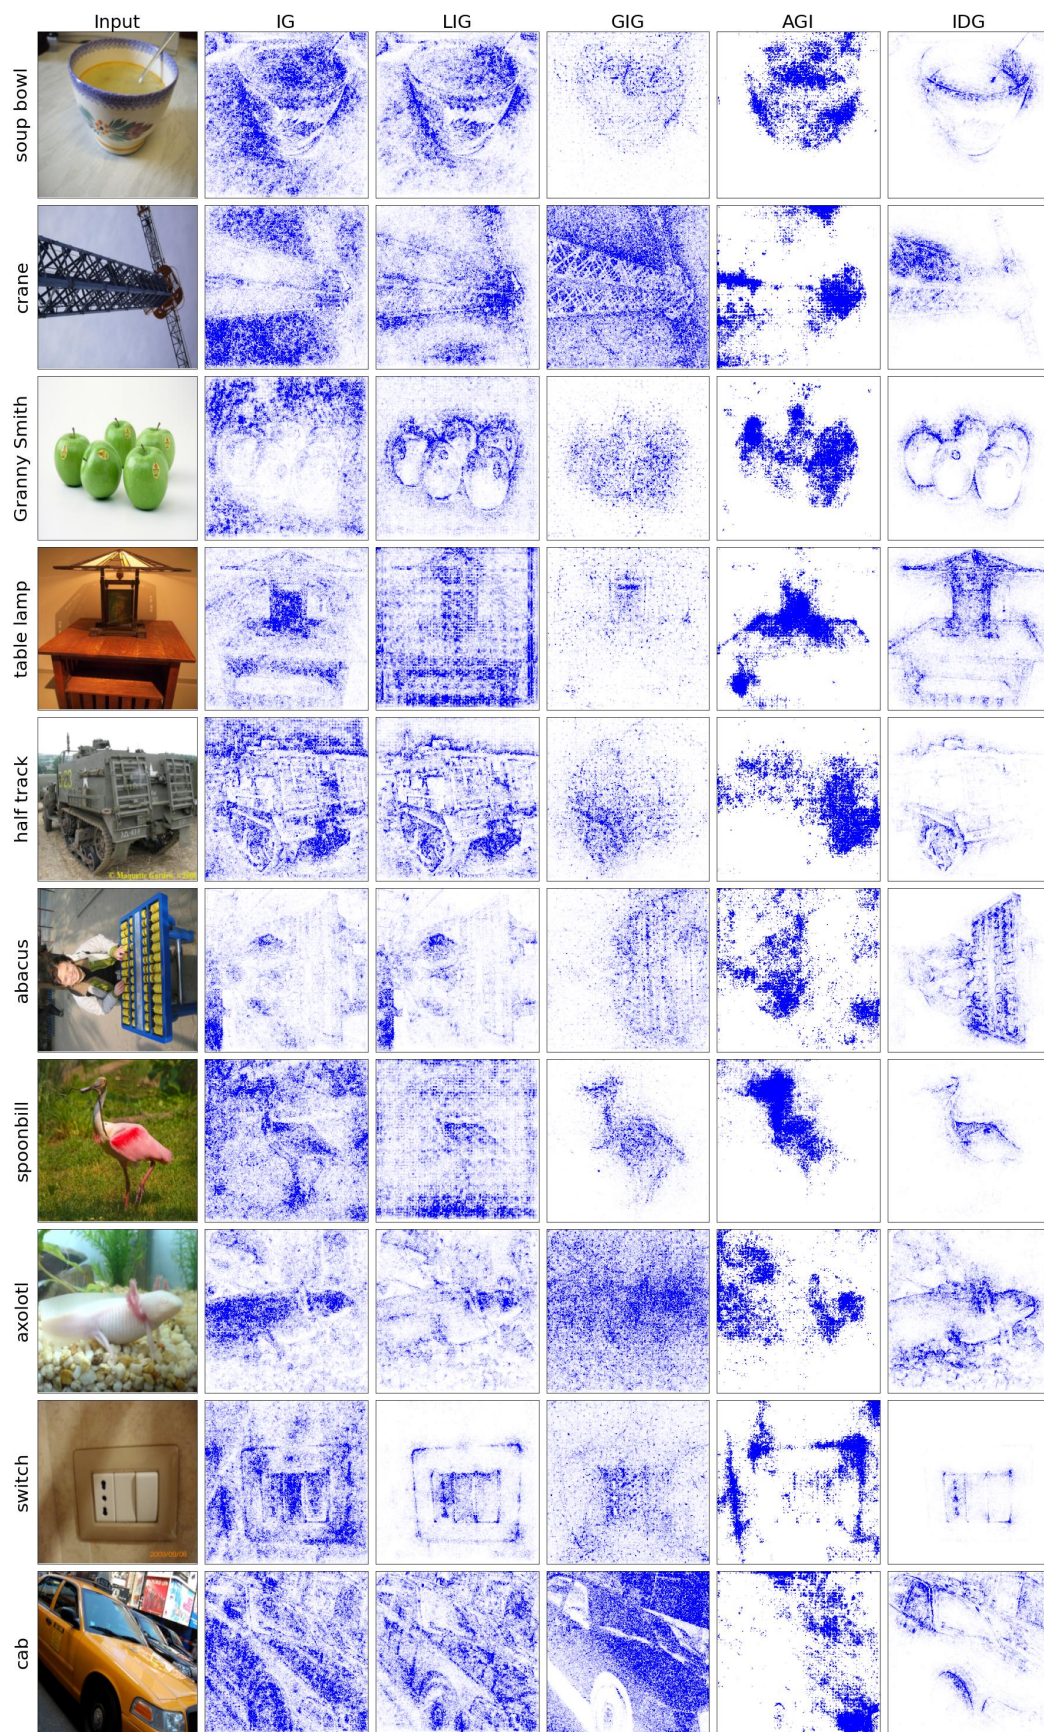



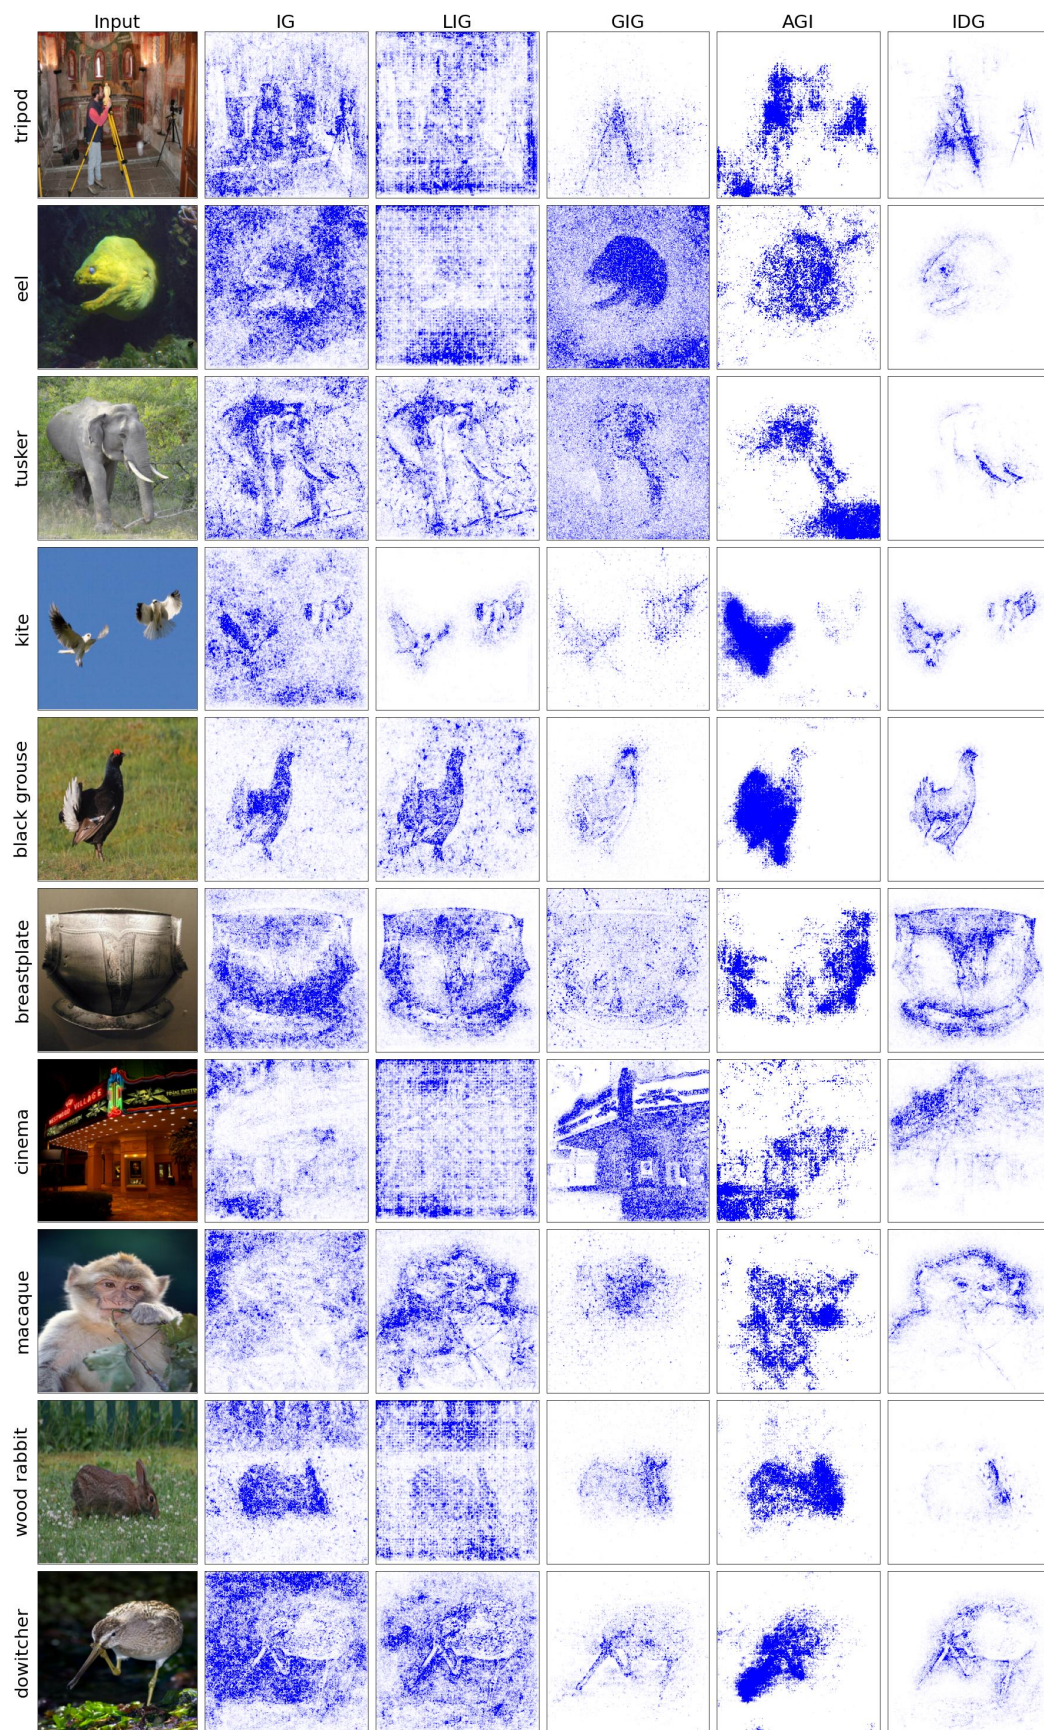



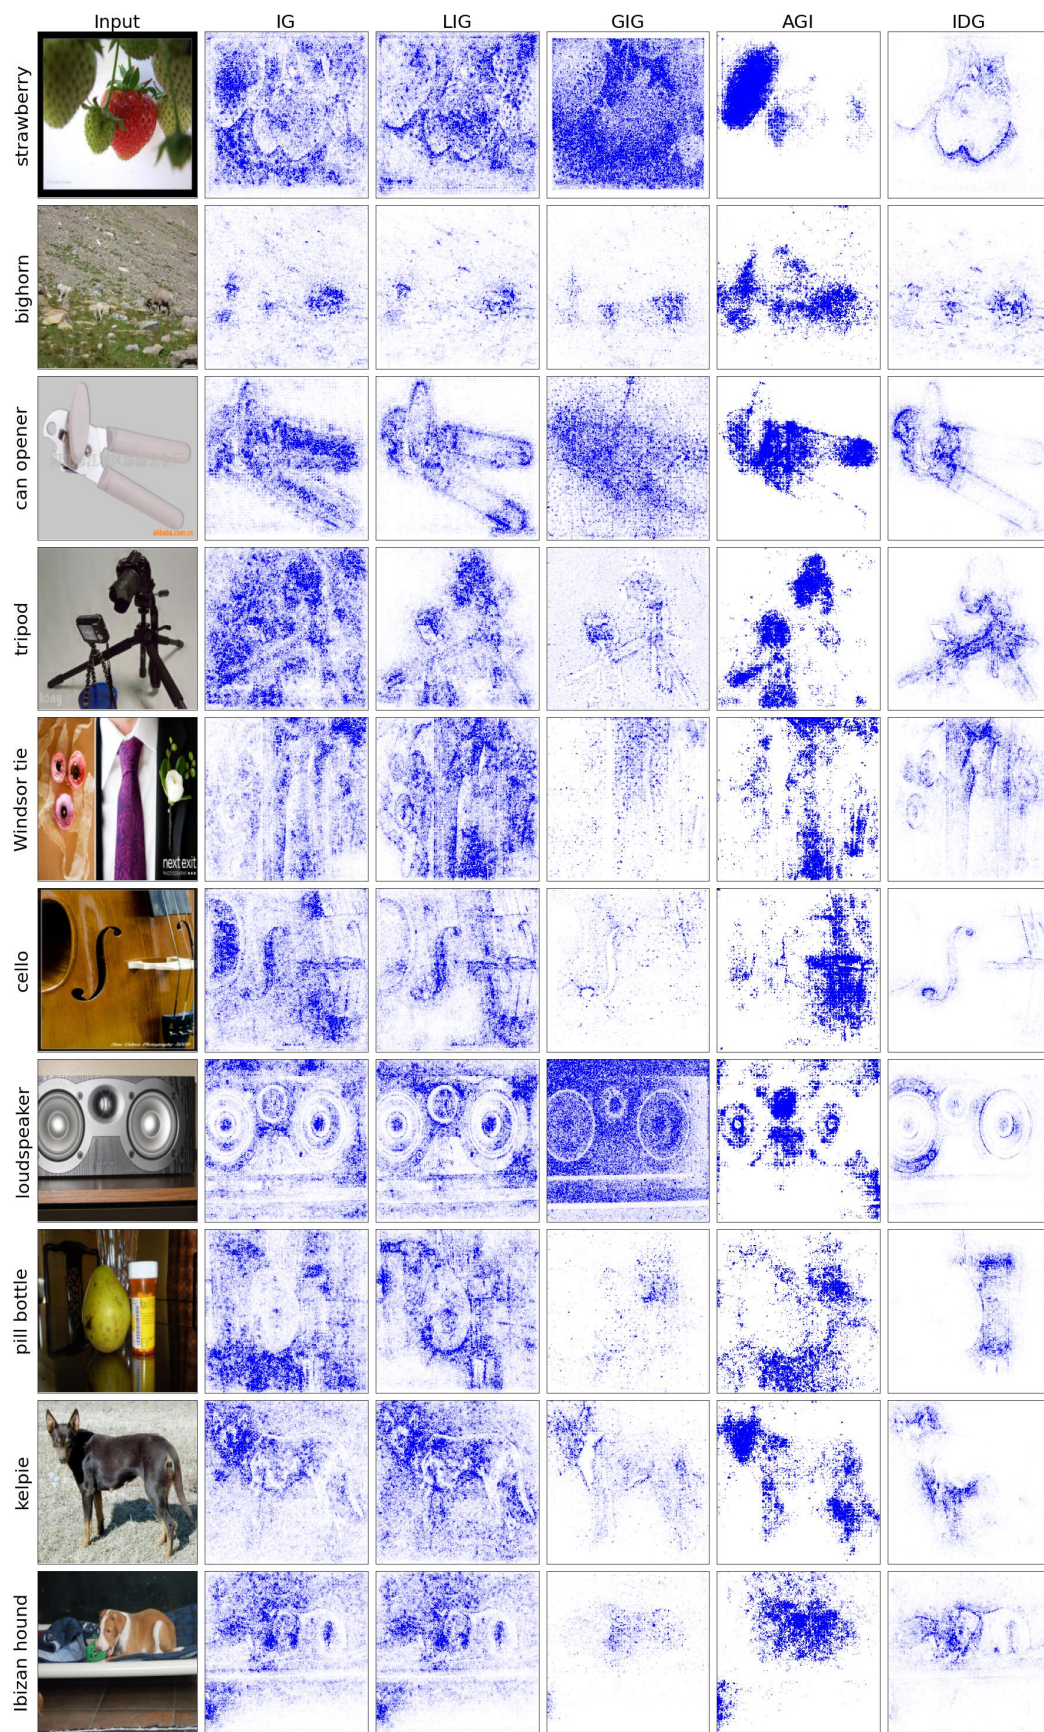



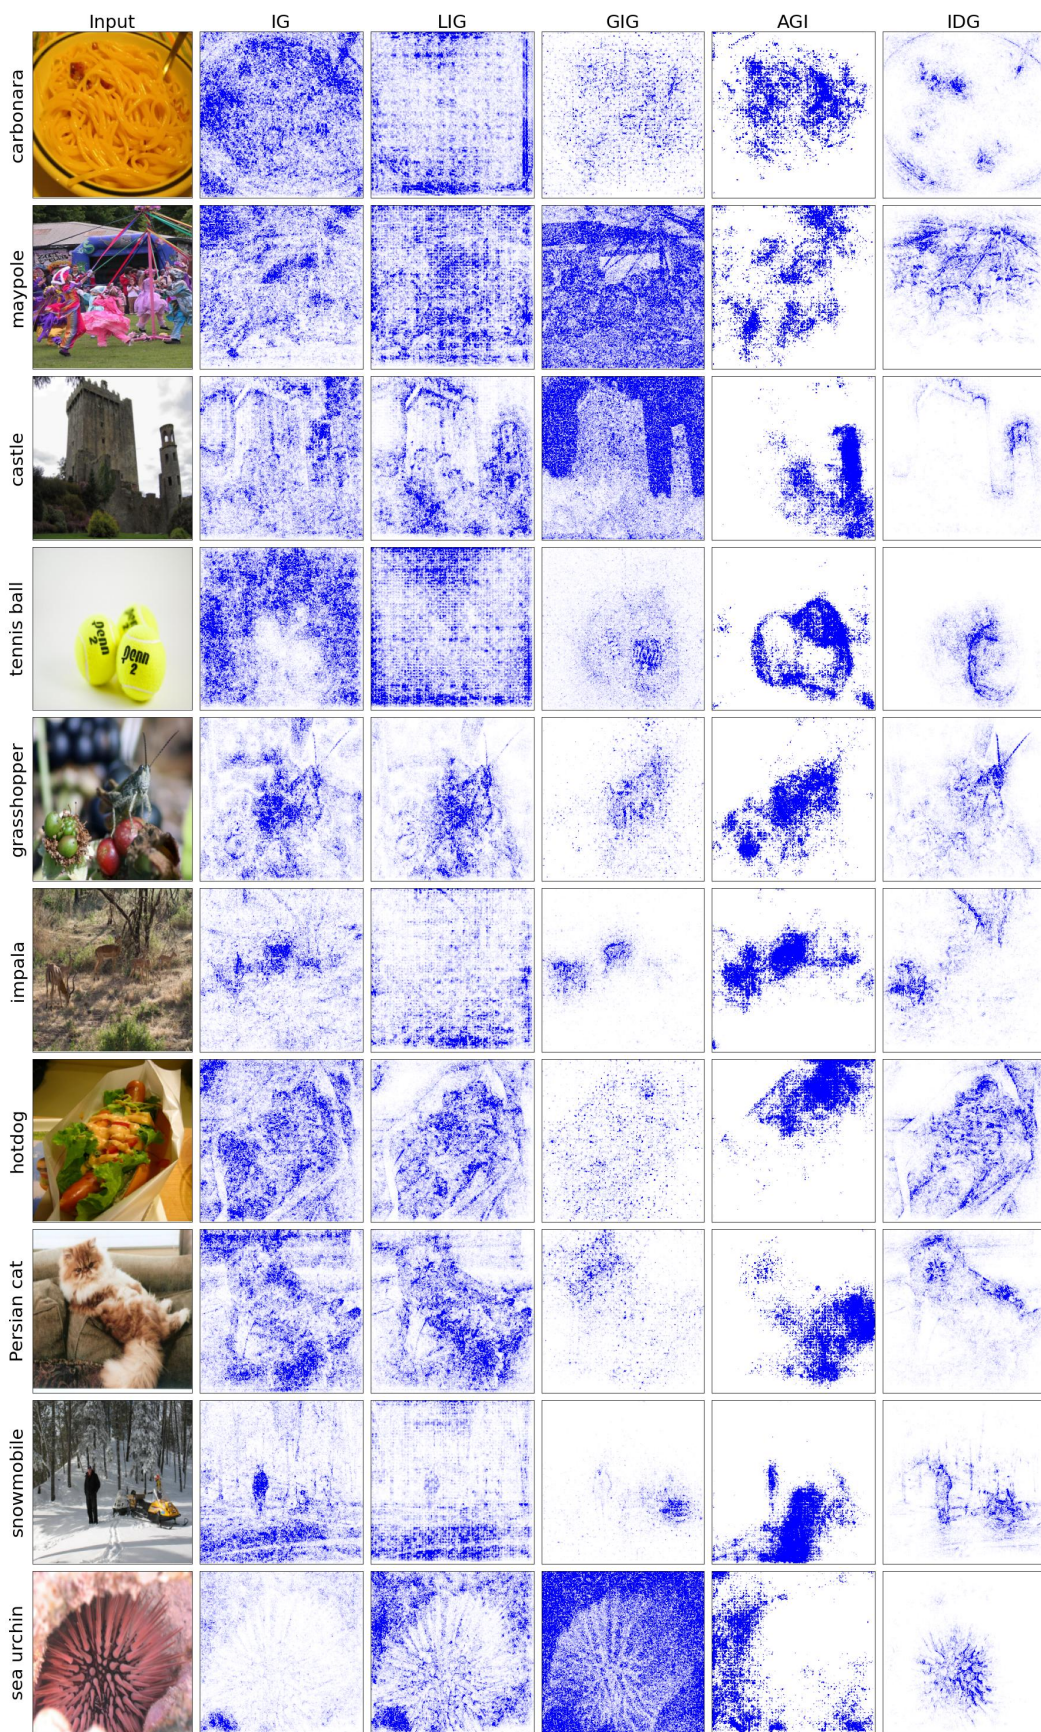



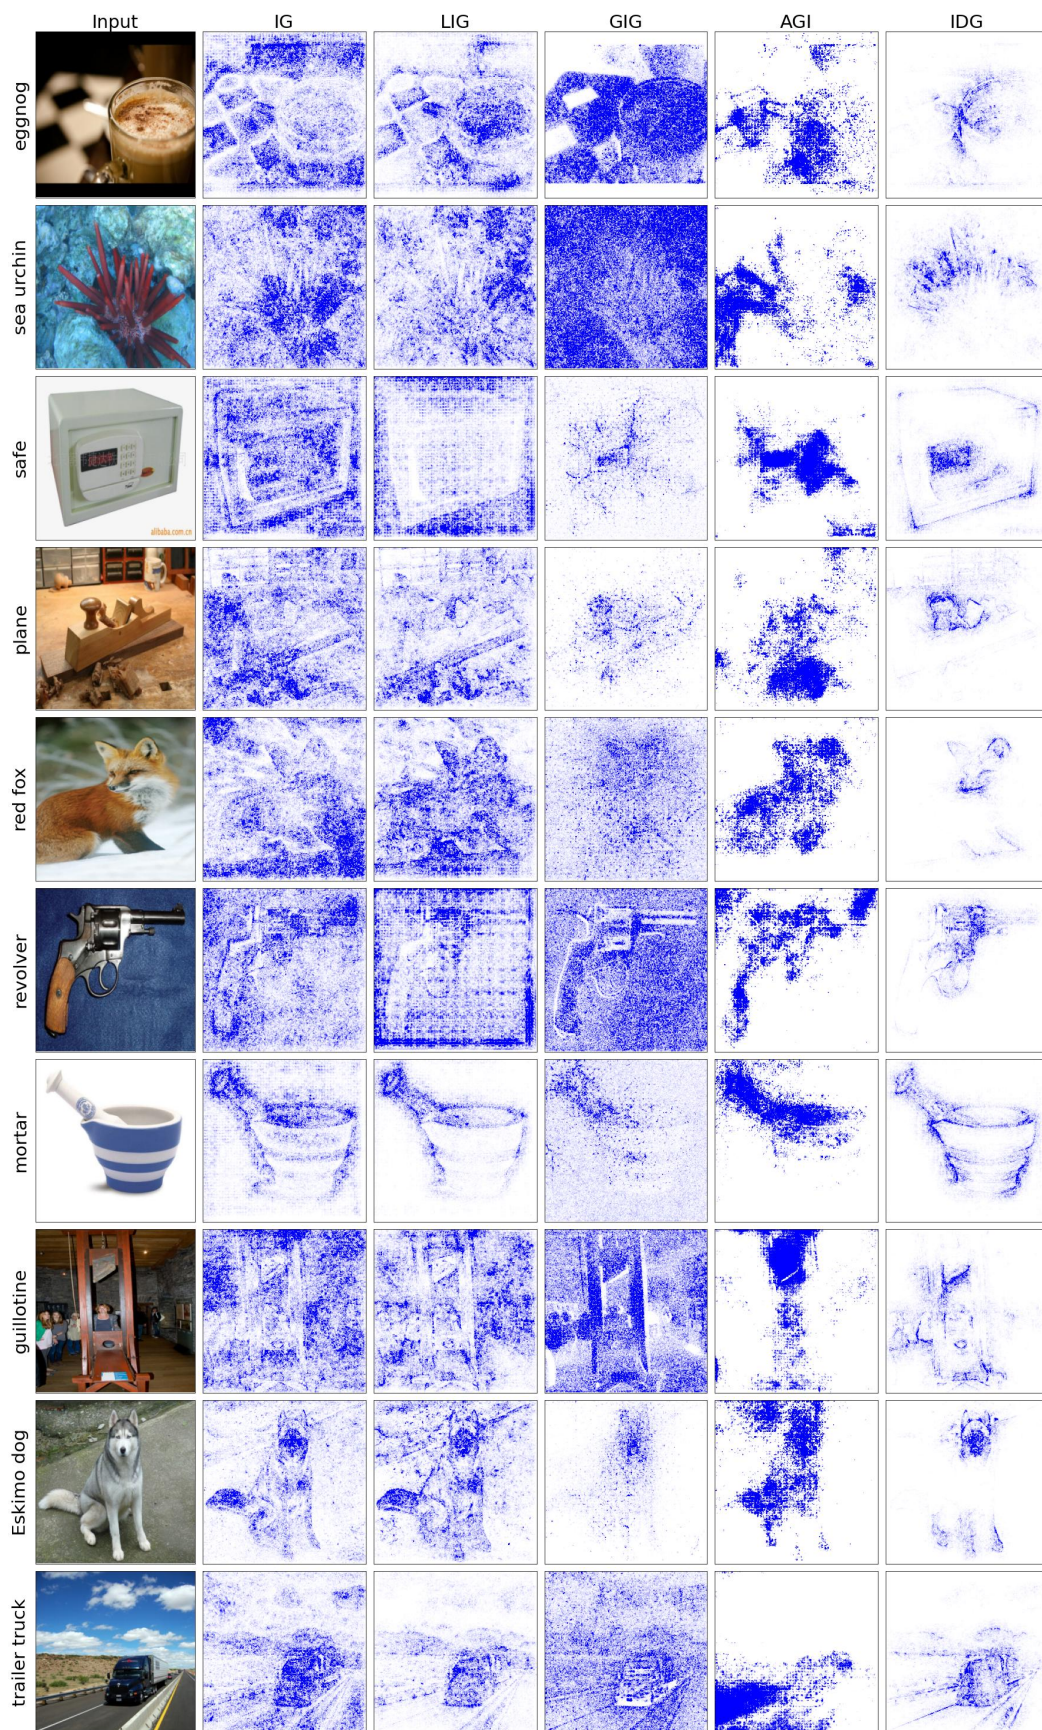

Supplement: Supplementary file 1 [file IDG_supplementary.pdf]
